# Supplementary material for: Doubled Shapiro steps in a dynamic axion insulator Josephson junction
Source: arXiv:2406.09274 source file (2024-06-13)
Supplement: Supplementary file 1 [file Supplementary_Information.pdf]

# Supplementary Information for "Doubled Shapiro steps in a dynamic axion insulator Josephson junction"

Yu-Hang Li[1,2,3], Ziqian Zhou[4], Ran Cheng[3,5], Hua Jiang[6] ✉, and X. C. Xie[4,6,7] ✉

[1] *School of Physics, Nankai University, Tianjin 300071, China*

[2] *State Key Laboratory of the Surface Physics and Department of Physics, Fudan University, Shanghai 200433, P. R. China*

[3] *Department of Electrical and Computer Engineering, University of California, Riverside, California 92521, USA*

[4] *International Center for Quantum Materials, School of Physics, Peking University, Beijing 100871, China*

[5] *Department of Physics and Astronomy, University of California, Riverside, California 92521, USA*

[6] *Interdisciplinary Center for Theoretical Physics and Information Sciences (ICTPIS), Fudan University, Shanghai 200433, China*

[7] *Hefei National Laboratory, Hefei 230088, China*

May 29, 2024

# Contents

**Note 1: Antiferromagnetic resonance of $Mn_2Bi_2Te_5$** **3**

* E-mail: jianghuaphy@fudan.edu.cn, xcxie@pku.edu.cn

**Note 2: Derivation of gauge invariant expression of the axion term.** **4**

**Note 3: Analytical expression for the dynamic axion field** **6**

## Note 1: Antiferromagnetic resonance of $Mn_2Bi_2Te_5$

In the macrospin approximation, the free energy for $Mn_2Bi_2Te_5$ is

$$F = -\lambda \mathbf{m}_1 \cdot \mathbf{m}_2 - H_A(m_{1z}^2 + m_{2z}^2) - H_0(m_{1z} + m_{2z}), \tag{1}$$

where $\mathbf{m}_{i=1,2} = \begin{bmatrix} m_{ix}, & m_{iy}, & m_{iz} \end{bmatrix}$ represents the antiparallel spin vector. The first term in Supplementary Eq. 1 describes the Heisenberg exchange interaction, the second term is the uniaxial anisotropy while the third term is the Zeeman energy in the presence of an external magnetic field along $\hat{z}$-direction. The effective magnetic fields acting on each spins are thus

$$\begin{aligned} \mathbf{H}_1^{eff} &= \frac{\partial F}{\partial \mathbf{m}_1} = \begin{bmatrix} -\lambda m_{2x}, & -\lambda m_{2y}, -\lambda m_{2z} - H_A m_{1z} - H_0 \end{bmatrix}, \\ \mathbf{H}_2^{eff} &= \frac{\partial F}{\partial \mathbf{m}_2} = \begin{bmatrix} -\lambda m_{1x}, & -\lambda m_{1y}, -\lambda m_{1z} - H_A m_{2z} - H_0 \end{bmatrix}. \end{aligned} \tag{2}$$

Substituting these effective magnetic field into the Landau–Lifshitz–Gilbert equation, we obtain

$$\begin{aligned} \frac{d\mathbf{m}_1}{dt} &= i\gamma \mathbf{m}_1 \times \mathbf{H}_1^{eff}, \\ \frac{d\mathbf{m}_2}{dt} &= i\gamma \mathbf{m}_2 \times \mathbf{H}_2^{eff}, \end{aligned} \tag{3}$$

where $\gamma$ is the gyromagnetic ratio. To solve Supplementary Eqs. 3, we assume $m_{1z} = -m_{2z} = 1$, and $m_{ix(y)} = w_{ix(y)} e^{-i\omega t}$. This further recasts the Landau–Lifshitz–Gilbert equation as [1]

$$\begin{bmatrix} 0, & 0, & -ia, & -ib \\ 0, & 0, & ib, & -id \\ ia, & ib, & 0, & 0 \\ -ib, & id, & 0, & 0 \end{bmatrix} \times \begin{bmatrix} w_{1x} \\ w_{2x} \\ w_{1y} \\ w_{2y} \end{bmatrix} = \omega \begin{bmatrix} w_{1x} \\ w_{2x} \\ w_{1y} \\ w_{2y}, \end{bmatrix} \tag{4}$$

where $a = \gamma(H_0 + H_A + H_E)$, $b = \gamma H_E$, $d = \gamma(H_0 - H_A - H_E)$. Diagonalizing this equation finally gives the eigenfrequency of the antiferromagnetic reasonance $\omega_\pm = \gamma(\sqrt{H_A(2H_E + H_A)} \pm$

$H_0$). In the absence of magnetic field, the eigenfrequency is $\omega = \gamma\sqrt{H_A(2H_E + H_A)}$. In $Mn_2Bi_2Te_5$, $H_A = 0.8$meV and $H_E = 0.1$meV, therefore the eigenfrequency is $f = \omega/2\pi \approx$ 143GHz.

## Note 2: Derivation of gauge invariant expression of the axion term.

For the low energy effective Hamiltonian of DAI with the form $\mathcal{H} = \sum_{i=1}^{5} d_i\Gamma^i$, it is straightforwardly to find that the eigenenergies are $E_\pm = \pm d$ with $d = \sqrt{(d_1^2 + d_2^2 + d_3^2 + d_4^2 + d_5^2)}$, and the corresponding eigenstates are

$$
\begin{aligned}
|\psi_+^1\rangle &= C_1\begin{pmatrix}-d_1 + id_2, & d_5 + id_3, & 0, & d + d_4\end{pmatrix}^{\mathrm{T}}, \\
|\psi_+^2\rangle &= C_1\begin{pmatrix}-d_5 + id_3, & -d_1 - id_1, & d + d_4, & 0\end{pmatrix}^{\mathrm{T}}, \\
|\psi_-^1\rangle &= C_2\begin{pmatrix}d_1 - id_2, & -d_5 - id_3, & 0, & d - d_4\end{pmatrix}^{\mathrm{T}}, \\
|\psi_-^2\rangle &= C_2\begin{pmatrix}d_5 - id_3, & d_1 + id_2, & d - d_4, & 0\end{pmatrix}^{\mathrm{T}},
\end{aligned} \tag{5}
$$

where $C_{1(2)} = 1/\sqrt{2d(d \pm d_4)}$ and $|\psi_\pm^{1,2}\rangle$ corresponds to $E_\pm$ respectively. As pointed out by Qi., *et. al.*, the gauge invariant expression for the axion field in condensed matter systems can be written in terms of the Chern-Simons 3-form

$$\theta = \frac{1}{4\pi}\int d^3\mathbf{k}\epsilon_{ijk}\mathrm{Tr}(A_i\partial_j A_k + i\frac{2}{3}A_iA_jA_k), \tag{6}$$

where $\epsilon_{ijk}$ is the Levi-Civita symbol and $A_j \equiv -i\sum_{\alpha\beta}\langle\psi_-^\alpha|\partial_j|\psi_-^\beta\rangle$ is the Berry connection defined on the occupied bands. Substituting the eigenstates in Supplementary Eq. 5 to

Supplementary Eq. 6, we obtain

$$\theta = -\frac{1}{4\pi}\sum_{\alpha\beta\gamma}\int d^3\mathbf{k}\epsilon_{ijk}(\langle\psi_-^\alpha|\partial_i\psi_-^\beta\rangle\langle\partial_j\psi_-^\beta|\partial_k\psi_-^\alpha\rangle + \frac{2}{3}\langle\psi_-^\alpha|\partial_i\psi_-^\beta\rangle\langle\psi_-^\beta|\partial_j\psi_-^\gamma\rangle\langle\psi_-^\gamma|\partial_k\psi_-^\alpha\rangle) \tag{7}$$

Using the relations

$$\begin{aligned}
&\epsilon_{ijk}\langle\psi_-^\alpha|\partial_i\psi_-^\alpha\rangle\langle\partial_j\psi_-^\alpha|\partial_k\psi_-^\alpha\rangle \\
&\quad = 2\epsilon_{ijk}C_1^4(d_2\partial_i d_1\partial_j d_3\partial_k d_5 - d_1\partial_i d_2\partial_j d_3\partial_k d_5 + d_5\partial_i d_3\partial_j d_1\partial_k d_2 - d_3\partial_i d_5\partial_j d_1\partial_k d_2), \\
&\sum_{\alpha\neq\beta}\epsilon_{ijk}\langle\psi_-^\alpha|\partial_i\psi_-^\beta\rangle\langle\partial_j\psi_-^\beta|\partial_k\psi_-^\alpha\rangle \\
&\quad = 4\epsilon_{ijk}C_1^4(d_1\partial_i d_5\partial_j d_3\partial_k d_2 - d_5\partial_i d_1\partial_j d_3\partial_k d_2 + d_2\partial_i d_3\partial_j d_5\partial_k d_1 - d_3\partial_i d_2\partial_j d_5\partial_k d_1) \\
&\quad + 4\epsilon_{ijk}C_1^2(d_3\partial_i d_1\partial_j d_5\partial_k d_2 - d_1\partial_i d_3\partial_j d_5\partial_k d_2 + d_2\partial_i d_5\partial_j d_1\partial_k d_3 - d_5\partial_i d_2\partial_j d_1\partial_k d_3), \\
&\sum_{\alpha\beta\gamma}\frac{2}{3}\langle\psi_-^\alpha|\partial_i\psi_-^\beta\rangle\langle\psi_-^\beta|\partial_j\psi_-^\gamma\rangle\langle\psi_-^\gamma|\partial_k\psi_-^\alpha\rangle \\
&\quad = 8\epsilon_{ijk}C_1^6(d-d_4^2)(d_2\partial_i d_1\partial_j d_3\partial_k d_5 - d_1\partial_i d_2\partial_j d_3\partial_k d_5 + d_5\partial_i d_3\partial_j d_1\partial_k d_2 - d_3\partial_i d_5\partial_j d_1\partial_k d_2),
\end{aligned} \tag{8}$$

we finally arrive at

$$\begin{aligned}
\theta &= \frac{1}{4\pi}\int d^3\mathbf{k}\epsilon_{ijk}\mathrm{Tr}(A_i\partial_j A_k + i\frac{2}{3}A_iA_jA_k) \\
&= -\frac{1}{4\pi}\sum_{\alpha\beta\gamma}\int d^3\mathbf{k}\epsilon_{ijk}(\langle\psi_-^\alpha|\partial_i\psi_-^\beta\rangle\langle\partial_j\psi_-^\beta|\partial_k\psi_-^\alpha\rangle + \frac{2}{3}\langle\psi_-^\alpha|\partial_i\psi_-^\beta\rangle\langle\psi_-^\beta|\partial_j\psi_-^\gamma\rangle\langle\psi_-^\gamma|\partial_k\psi_-^\alpha\rangle) \\
&= \frac{1}{4\pi}\int d^3\mathbf{k}[12C_1^4 - 8C_1^6(d^2-d_4^2)]\epsilon_{ijkl}d_i\partial_x d_j\partial_y d_k\partial_z d_l \\
&= \frac{1}{4\pi}\int d^3\mathbf{k}\left[\frac{3}{d^2(d+d_4)^2} - \frac{d-d_4}{d^3(d+d_4)^2}\right]\epsilon_{ijkl}d_i\partial_x d_j\partial_y d_k\partial_z d_l \\
&= \frac{1}{4\pi}\int d^3\mathbf{k}\frac{2d+d_4}{d^3(d+d_4)^2}\epsilon_{ijkl}d_i\partial_x d_j\partial_y d_k\partial_z d_l.
\end{aligned} \tag{9}$$

# Note 3: Analytical expression for the dynamic axion field

As stated in the main text, the dynamic axion field in the presence of an antiferromagnetic resonance can be calculated adiabatically by using

$$\theta(t) = -\frac{1}{4\pi}\int d\boldsymbol{k}^3 \frac{2d(t)+d_4}{[d(t)+d_4]^2 d(t)^3} d_5(t)\partial_{k_x}d_1\partial_{k_y}d_2\partial_{k_z}d_3, \tag{10}$$

where $d_5 = m_5\sqrt{1-A_x^2\sin^2\omega t}$. Here, all parameters are the same as those defined in the main text. Since $A_x \ll 1$ is a small variable, Supplementary equation 10 can thus be expanded perturbatively. We then obtain

$$\begin{aligned}\theta(t) =& \frac{m_5(m_4+2m)}{m^3(m_4+m)^2} + \frac{m_5(9mm_4m_5^2+8m^2m_5^2+3m_4^2m_5^2-m^2m_4^2-3m^4-2m^3m_4)}{2m^5(m_4+m)^3}A_x^2\sin^2\omega t \\ &+\mathcal{O}(A_x^2\sin^2\omega t),\end{aligned} \tag{11}$$

where $m_{1,2,3,4} = d_{1,2,3,4}$, $m^2 = \sum_{i=1}^5 m_i^2$ and $\mathcal{O}(x)$ is the higher order term. It is apparently from Supplementary Eq. 11 that the frequency of the dynamic part of the axion field is doubled under the driven of a microwave, or $\omega_\theta = 2\omega$.

# Supplementary References


[1] F. Keffer and C. Kittel, *Phys. Rev.* **85**, 329 (1952)

[2] I. S. Gradshteyn, I. M. Ryzhik, Table of Integrals: 8.511 3.
